# Supplementary material for: Moments and Root-Mean-Square Error of the Bayesian MMSE Estimator of Classification Error in the Gaussian Model
Source: arXiv:1310.1519 source file (2013-11-12)
Supplement: Supplementary file 1 [file SupplementaryMaterials.pdf]

# Moments and Root-Mean-Square Error of the Bayesian MMSE Estimator of Classification Error in the Gaussian Model – Supplementary Materials


Amin Zollanvari[a,b,*], Edward R. Dougherty[a,c]

[a] *Department of Electrical and Computer Engineering, Texas A&M University, College Station, TX 77843*
[b] *Department of Statistics, Texas A&M University, College Station, TX 77843*
[c] *Translational Genomics Research Institute (TGEN), Phoenix, AZ 85004*


## 1. Proofs

### Section A: Proof of Equation (22)

We need to find the right-hand side of (21). We have already found the value of the numerator, $E_{S_n,\mathbf{z}}[U_0(\bar{\mathbf{x}}_0, \bar{\mathbf{x}}_1, \mathbf{z}) \leq 0 | \mathbf{z} \in \Psi_0, \boldsymbol{\mu})]$, in deriving Theorem 1. Indeed, the numerator is the same as (18). To find $\mathrm{Var}_{S_n,\mathbf{z}}[U_0(\bar{\mathbf{x}}_0, \bar{\mathbf{x}}_1, \mathbf{z}) \leq 0 | \mathbf{z} \in \Psi_0, \boldsymbol{\mu}]$, we first represent $U_0(\bar{\mathbf{x}}_0, \bar{\mathbf{x}}_1, \mathbf{z})$ as a quadratic form:

$$U_0(\bar{\mathbf{x}}_0, \bar{\mathbf{x}}_1, \mathbf{z}) = \frac{1}{2}\mathbf{y}^T\mathbf{C}\mathbf{y},$$

where $\mathbf{y}$ is a vector of size $(n_0 + n_1)p$ obtained by stacking all observations and the random vector $\mathbf{z}$,

$$\begin{aligned} \mathbf{y} &= \left[\mathbf{z}^T, \mathbf{x}_1^T, \ldots, \mathbf{x}_{n_0}^T, \mathbf{x}_{n_0+1}^T, \ldots, \mathbf{x}_{n_0+n_1}^T\right]^T, \\ \mathbf{C} &= \mathbf{H_B} \otimes \mathbf{\Sigma}^{-1}, \end{aligned}$$

where $\otimes$ denotes the Kronecker product of two matrices, with

$$\mathbf{H_B} = \frac{1}{2}\begin{bmatrix} 0 & \frac{\nu_0 \mathbf{1}_{n_0}^T}{n_0(n_0+\nu_0)} & \frac{-\nu_0 \mathbf{1}_{n_1}^T}{n_1(n_0+\nu_0)} \\ \frac{\nu_0 \mathbf{1}_{n_0}}{n_0(n_0+\nu_0)} & \frac{(n_0-\nu_0)\mathbf{1}_{n_0\times n_0}}{n_0^2(n_0+\nu_0)} & \frac{-\mathbf{1}_{n_0\times n_1}}{n_1(n_0+\nu_0)} \\ \frac{-\nu_0 \mathbf{1}_{n_1}}{n_1(n_0+\nu_0)} & \frac{-\mathbf{1}_{n_1\times n_0}}{n_1(n_0+\nu_0)} & \frac{\mathbf{1}_{n_1\times n_1}}{n_1^2} \end{bmatrix},$$

where $\mathbf{a}_{k\times l}$ is a matrix of size $k \times l$ and $\mathbf{a}_k$ is a column vector of size $k$, with all elements being "a". From [1], we see that for, $\mathbf{y} \sim N(\boldsymbol{\mu}, \mathbf{\Sigma})$ and a real symmetric positive definite matrix $\mathbf{A}$,

$$\mathrm{Var}[\mathbf{y}^T\mathbf{A}\mathbf{y}] = 2tr(\mathbf{A}\mathbf{\Sigma})^2 + 4\boldsymbol{\mu}^T\mathbf{A}\mathbf{\Sigma}\mathbf{A}\boldsymbol{\mu}\,,$$

with $tr$ being the trace operator. Therefore,

$$\begin{aligned} \mathrm{Var}_{S_n,\mathbf{z}}[U_0(\bar{\mathbf{x}}_0, \bar{\mathbf{x}}_1, \mathbf{z}) \leq 0 | \mathbf{z} \in \Psi_0, \boldsymbol{\mu}] = &\frac{1}{2}tr\left(\mathbf{H_B}\mathbf{I}'_{n_0+n_1+1}\mathbf{H_B}\mathbf{I}'_{n_0+n_1+1} \otimes \mathbf{I}_p\right) \\ &+ \boldsymbol{\phi}^T(\mathbf{H_B}\mathbf{I}'_{n_0+n_1+1}\mathbf{H_B} \otimes \mathbf{\Sigma}^{-1})\boldsymbol{\phi}\,, \end{aligned}$$


*Corresponding author.
*Email addresses:* amin_zoll@neo.tamu.edu (Amin Zollanvari), edward@ece.tamu.edu (Edward R. Dougherty)

where $\mathbf{I}_p$ is the identity matrix of size $p$, $\mathbf{I}'_{n_0+n_1+1}$ is obtained from the identity matrix of $\mathbf{I}_{n_0+n_1+1}$ by replacing the first diagonal element on the top left corner with $\frac{(n_0+\nu_0+1)(n_0+\nu_0)}{\nu_0^2}$, and

$$\boldsymbol{\phi} = [0, \mathbf{1}_{n_0}^T, \mathbf{0}_{n_0}^T]^T \otimes \boldsymbol{\mu}_0 + [0, \mathbf{0}_{n_0}^T, \mathbf{1}_{n_0}^T]^T \otimes \boldsymbol{\mu}_1 + [1, \mathbf{0}_{n_0}^T, \mathbf{0}_{n_0}^T]^T \otimes \mathbf{m}_0.$$

Some algebraic manipulations yield

$$\begin{aligned}
D_0^{B,R} &= \left(\frac{n_0+\nu_0+1}{n_0+\nu_0} + \frac{n_0}{(n_0+\nu_0)^2} + \frac{1}{n_1}\right)\boldsymbol{\mu}_1^T\boldsymbol{\Sigma}^{-1}\boldsymbol{\mu}_1 \\
&+ \left(\frac{n_0+\nu_0+1}{n_0+\nu_0} + \frac{(n_0-\nu_0)^2}{n_0(n_0+\nu_0)^2} + \frac{n_0^2}{n_1(n_0+\nu_0)^2}\right)\boldsymbol{\mu}_0^T\boldsymbol{\Sigma}^{-1}\boldsymbol{\mu}_0 \\
&-2\left(\frac{n_0+\nu_0+1}{n_0+\nu_0} + \frac{n_0-\nu_0}{(n_0+\nu_0)^2} + \frac{n_0}{n_1(n_0+\nu_0)}\right)\boldsymbol{\mu}_0^T\boldsymbol{\Sigma}^{-1}\boldsymbol{\mu}_1 \\
&+2\left(\frac{\nu_0(n_0-\nu_0)}{n_0(n_0+\nu_0)^2} + \frac{\nu_0 n_0}{n_1(n_0+\nu_0)^2}\right)\mathbf{m}_0^T\boldsymbol{\Sigma}^{-1}\boldsymbol{\mu}_0 \\
&-2\left(\frac{\nu_0}{(n_0+\nu_0)^2} + \frac{\nu_0}{n_1(n_0+\nu_0)}\right)\mathbf{m}_0^T\boldsymbol{\Sigma}^{-1}\boldsymbol{\mu}_1 \\
&+\frac{\nu_0^2}{(n_0+\nu_0)^2}\left(\frac{1}{n_0} + \frac{1}{n_1}\right)\mathbf{m}_0^T\boldsymbol{\Sigma}^{-1}\mathbf{m}_0 \\
&+\frac{n_0+\nu_0+1}{n_0+\nu_0}\left(\frac{p}{n_0} + \frac{p}{n_1}\right) + \frac{(n_0-\nu_0)^2 p}{2n_0^2(n_0+\nu_0)^2} + \frac{n_0 p}{n_1(n_0+\nu_0)^2} + \frac{p}{2n_1^2},
\end{aligned}$$

which can be shown to be equivalent to the result in (24).

## Section B: Proof of Equation (33)

We first introduce some identities. We can show that for $\boldsymbol{\mu}_i \sim N(\mathbf{m}_i, \boldsymbol{\Sigma}/\nu_i)$,

$$\begin{aligned}
\mathrm{Var}_{\boldsymbol{\mu}}[\boldsymbol{\mu}_i^T\boldsymbol{\Sigma}^{-1}\boldsymbol{\mu}_i] &= 2\frac{p}{\nu_i^2} + 4\frac{\mathbf{m}_i^T\boldsymbol{\Sigma}^{-1}\mathbf{m}_i}{\nu_i}, \\
\mathrm{Var}_{\boldsymbol{\mu}}(\boldsymbol{\mu}_i^T\boldsymbol{\Sigma}^{-1}\boldsymbol{\mu}_j) &= \frac{p}{\nu_i\nu_j} + \frac{\mathbf{m}_i^T\boldsymbol{\Sigma}^{-1}\mathbf{m}_i}{\nu_j} + \frac{\mathbf{m}_j^T\boldsymbol{\Sigma}^{-1}\mathbf{m}_j}{\nu_i} \\
\mathrm{Cov}_{\boldsymbol{\mu}}[\mathbf{a}^T\boldsymbol{\mu}_i,\ \boldsymbol{\mu}_i^T\boldsymbol{\Sigma}^{-1}\boldsymbol{\mu}_i] &= \frac{2}{\nu_i}\mathbf{a}^T\mathbf{m}_i \\
\mathrm{Cov}_{\boldsymbol{\mu}}[\boldsymbol{\mu}_j^T\boldsymbol{\Sigma}^{-1}\boldsymbol{\mu}_i,\ \boldsymbol{\mu}_i^T\boldsymbol{\Sigma}^{-1}\boldsymbol{\mu}_i] &= \frac{2}{\nu_i}\mathbf{m}_j^T\boldsymbol{\Sigma}^{-1}\mathbf{m}_i
\end{aligned} \tag{S.1}$$

and

$$\begin{aligned}
E_{\boldsymbol{\mu}}[\boldsymbol{\mu}_i^T\boldsymbol{\Sigma}^{-1}\boldsymbol{\mu}_i] &= \mathbf{m}_i^T\boldsymbol{\Sigma}^{-1}\mathbf{m}_i + \frac{p}{\nu_i}, \\
E_{\boldsymbol{\mu}}[\boldsymbol{\mu}_i^T\boldsymbol{\Sigma}^{-1}\boldsymbol{\mu}_j] &= \mathbf{m}_i^T\boldsymbol{\Sigma}^{-1}\mathbf{m}_j, i \neq j.
\end{aligned} \tag{S.2}$$

To find the numerator of (32), $E_{\boldsymbol{\mu},S_n,\mathbf{z}}[U_0(\bar{\mathbf{x}}_0, \bar{\mathbf{x}}_1, \mathbf{z})|\mathbf{z} \in \Psi_0)]$, we note that we have already computed $E_{S_n,\mathbf{z}}[U_0(\bar{\mathbf{x}}_0, \bar{\mathbf{x}}_1, \mathbf{z})|\mathbf{z} \in \Psi_0, \boldsymbol{\mu})]$ to obtain (22) from (21). Therefore, using identities (S.2), we get

$$E_{\boldsymbol{\mu},S_n,\mathbf{z}}[U_0(\bar{\mathbf{x}}_0, \bar{\mathbf{x}}_1, \mathbf{z})|\mathbf{z} \in \Psi_0)] = E_{\boldsymbol{\mu}}[G_0^{B,R}] = H_0^R,$$

with $G_0^{B,R}$ and $H_0^R$ presented in (23) and (31), respectively. For the denominator of (32), we have

$$\begin{aligned}
&\mathrm{Var}_{\boldsymbol{\mu},S_n,\mathbf{z}}[U_0(\bar{\mathbf{x}}_0,\bar{\mathbf{x}}_1,\mathbf{z})|\mathbf{z}\in\Psi_0]\\
&=\mathrm{Var}_{\boldsymbol{\mu}}\big[E_{S_n,\mathbf{z}}[U_0(\bar{\mathbf{x}}_0,\bar{\mathbf{x}}_1,\mathbf{z})|\boldsymbol{\mu},\mathbf{z}\in\Psi_0]\big]\\
&+E_{\boldsymbol{\mu}}\big[\mathrm{Var}_{S_n,\mathbf{z}}[U_0(\bar{\mathbf{x}}_0,\bar{\mathbf{x}}_1,\mathbf{z})|\boldsymbol{\mu},\mathbf{z}\in\Psi_0]\big]\\
&=\mathrm{Var}_{\boldsymbol{\mu}}[G_0^{B,R}]+E_{\boldsymbol{\mu}}[D_0^{B,R}]
\end{aligned} \tag{S.3}$$

with $G_0^{B,R}$ and $D_0^{B,R}$ presented in (23) and (24), respectively. Using identities (S.1), we can show that the first summand on the right-hand side of (S.3) is

$$\begin{aligned}
\mathrm{Var}_{\boldsymbol{\mu}}[G_0^{B,R}]&=\mathbf{m}_0^T\boldsymbol{\Sigma}^{-1}\mathbf{m}_0\left(\frac{1}{\nu_0(1+\frac{\nu_0}{n_0})^2}+\frac{1}{\nu_1}\right)\\
&+\frac{\mathbf{m}_1^T\boldsymbol{\Sigma}^{-1}\mathbf{m}_1}{\nu_1}+\frac{\mathbf{m}_1^T\boldsymbol{\Sigma}^{-1}\mathbf{m}_1}{\nu_0(1+\frac{\nu_0}{n_0})^2}-\frac{2\mathbf{m}_0^T\boldsymbol{\Sigma}^{-1}\mathbf{m}_1}{\nu_0(1+\frac{\nu_0}{n_0})^2}-\frac{2\mathbf{m}_0^T\boldsymbol{\Sigma}^{-1}\mathbf{m}_1}{\nu_1(1+\frac{\nu_0}{n_0})}\\
&+\frac{(n_0-\nu_0)^2p}{2\nu_0^2(n_0+\nu_0)^2}+\frac{n_0^2p}{\nu_0\nu_1(n_0+\nu_0)^2}+\frac{p}{2\nu_1^2},
\end{aligned} \tag{S.4}$$

To find the second summand, $E_{\boldsymbol{\mu}}[D_0^{B,R}]$, we use (S.2). We get $\mathrm{Var}_{\boldsymbol{\mu}}[G_0^{B,R}]+E_{\boldsymbol{\mu}}[D_0^{B,R}]\triangleq F_0^R$, with $F_0^R$ defined in (34).

**Section C: Proof of Equation (56)**

Owing to the identities in (S.1),

$$\begin{aligned}
C_{01}^{B,R}&=-\mathrm{Cov}_{S_n,\mathbf{z}}[U_0(\bar{\mathbf{x}}_0,\bar{\mathbf{x}}_1,\mathbf{z}),U_1(\bar{\mathbf{x}}_0,\bar{\mathbf{x}}_1,\mathbf{z}')|\mathbf{z}\in\Psi_0,\mathbf{z}'\in\Psi_1,\boldsymbol{\mu}]\\
&=\frac{p}{(n_0+\nu_0)(n_1+\nu_1)}+\frac{(n_0-\nu_0)p}{2n_0^2(n_0+\nu_0)}+\frac{(n_1-\nu_1)p}{2n_1^2(n_1+\nu_1)}\\
&+\frac{\boldsymbol{\mu}_0^T\boldsymbol{\Sigma}^{-1}\boldsymbol{\mu}_1}{(n_0+\nu_0)(n_1+\nu_1)}\left(\frac{n_0\nu_1}{n_1}+\frac{n_1\nu_0}{n_0}-\nu_0-\nu_1-2n_0-2n_1\right)\\
&+\frac{\boldsymbol{\mu}_0^T\boldsymbol{\Sigma}^{-1}\boldsymbol{\mu}_0}{n_0+\nu_0}\left(1+\frac{n_0}{n_1+\nu_1}-\frac{\nu_0}{n_0}\right)+\frac{\boldsymbol{\mu}_1^T\boldsymbol{\Sigma}^{-1}\boldsymbol{\mu}_1}{n_1+\nu_1}\left(1+\frac{n_1}{n_0+\nu_0}-\frac{\nu_1}{n_1}\right)\\
&+\frac{\nu_0(n_0+n_1+\nu_1)\mathbf{m}_0^T\boldsymbol{\Sigma}^{-1}\boldsymbol{\mu}_0}{n_0(n_0+\nu_0)(n_1+\nu_1)}+\frac{\nu_1(n_0+n_1+\nu_0)\mathbf{m}_1^T\boldsymbol{\Sigma}^{-1}\boldsymbol{\mu}_1}{n_1(n_0+\nu_0)(n_1+\nu_1)}\\
&+\frac{\nu_0\left(\frac{\nu_1}{n_1}-\frac{n_1}{n_0}-1\right)\mathbf{m}_0^T\boldsymbol{\Sigma}^{-1}\boldsymbol{\mu}_1}{(n_0+\nu_0)(n_1+\nu_1)}+\frac{\nu_1\left(\frac{\nu_0}{n_0}-\frac{n_0}{n_1}-1\right)\mathbf{m}_1^T\boldsymbol{\Sigma}^{-1}\boldsymbol{\mu}_0}{(n_0+\nu_0)(n_1+\nu_1)}\\
&-\frac{\nu_0\nu_1}{(n_0+\nu_0)(n_1+\nu_1)}\left(\frac{1}{n_0}+\frac{1}{n_1}\right)\mathbf{m}_0^T\boldsymbol{\Sigma}^{-1}\mathbf{m}_1.
\end{aligned}$$

After some algebraic simplifications and matching the terms properly, we get the result stated in (56).

**Section D: Proof of Equation (75)**

We use the law of total covariance to find $K_0^{B,R}$ as follows:

$$\begin{aligned}K_0^{B,R} &= \mathrm{Cov}_{\boldsymbol{\mu},S_n,\mathbf{z}}[U_0(\bar{\mathbf{x}}_0,\bar{\mathbf{x}}_1,\mathbf{z}),U_0(\bar{\mathbf{x}}_0,\bar{\mathbf{x}}_1,\mathbf{z}')|\mathbf{z}\in\Psi_0,\mathbf{z}'\in\Psi_0] \\ &= \mathrm{Cov}_{\boldsymbol{\mu}}\left[E_{S_n,\mathbf{z}}[U_0(\bar{\mathbf{x}}_0,\bar{\mathbf{x}}_1,\mathbf{z})|\boldsymbol{\mu},\mathbf{z}\in\Psi_0],E_{S_n,\mathbf{z}'}[U_0(\bar{\mathbf{x}}_0,\bar{\mathbf{x}}_1,\mathbf{z}')|\boldsymbol{\mu},\mathbf{z}'\in\Psi_0]\right] \\ &+E_{\boldsymbol{\mu}}\left[\mathrm{Cov}_{S_n,\mathbf{z}}[U_0(\bar{\mathbf{x}}_0,\bar{\mathbf{x}}_1,\mathbf{z}),U_0(\bar{\mathbf{x}}_0,\bar{\mathbf{x}}_1,\mathbf{z}')|\mathbf{z}\in\Psi_0,\mathbf{z}'\in\Psi_0,\boldsymbol{\mu}]\right] = \mathrm{Var}_{\boldsymbol{\mu}}[G_0^{B,R}]+E_{\boldsymbol{\mu}}[C_0^{B,R}]\,,\end{aligned}$$

where $G_0^{B,R}$ and $C_0^{B,R}$ are defined in (23) and (53), respectively. Note that $\mathrm{Var}_{\boldsymbol{\mu}}[G_0^{B,R}]$ appears in the last equality due to independence of $\mathbf{z}$ and $\mathbf{z}'$ and having $E_{S_n,\mathbf{z}}[U_0(\bar{\mathbf{x}}_0,\bar{\mathbf{x}}_1,\mathbf{z})|\mathbf{z}\in\Psi_0,\boldsymbol{\mu})] = G_0^{B,R}$ from (23). Now, $\mathrm{Var}_{\boldsymbol{\mu}}[G_0^{B,R}]$ is already obtained in (S.4) and $E_{\boldsymbol{\mu}}[C_0^{B,R}]$ is easily computed from identities in (S.2). Some algebraic manipulations then yield (75).

**Section E: Proof of Equation (78)**

As in Section D, the law of total covariance yields

$$\begin{aligned}K_{01}^{B,R} &= \mathrm{Cov}_{\boldsymbol{\mu},S_n,\mathbf{z}}[U_0(\bar{\mathbf{x}}_0,\bar{\mathbf{x}}_1,\mathbf{z}),-U_1(\bar{\mathbf{x}}_0,\bar{\mathbf{x}}_1,\mathbf{z}')\,|\,\mathbf{z}\in\Psi_0,\mathbf{z}'\in\Psi_1] \\ &= -\mathrm{Cov}_{\boldsymbol{\mu}}\left[E_{S_n,\mathbf{z}}[U_0(\bar{\mathbf{x}}_0,\bar{\mathbf{x}}_1,\mathbf{z})|\boldsymbol{\mu},\mathbf{z}\in\Psi_0],E_{S_n,\mathbf{z}'}[U_1(\bar{\mathbf{x}}_0,\bar{\mathbf{x}}_1,\mathbf{z}')|\boldsymbol{\mu},\mathbf{z}'\in\Psi_1]\right] \\ &- E_{\boldsymbol{\mu}}\left[\mathrm{Cov}_{S_n,\mathbf{z}}[U_0(\bar{\mathbf{x}}_0,\bar{\mathbf{x}}_1,\mathbf{z}),U_1(\bar{\mathbf{x}}_0,\bar{\mathbf{x}}_1,\mathbf{z}')\,|\,\mathbf{z}\in\Psi_0,\mathbf{z}'\in\Psi_1,\boldsymbol{\mu}]\right] \\ &= -\mathrm{Cov}_{\boldsymbol{\mu}}[G_0^{B,R},G_1^{B,R}]+E_{\boldsymbol{\mu}}[C_{01}^{B,R}]\end{aligned} \tag{S.5}$$

The last equality follows from the preceding sum because the expectations inside the covariance in the first summand are, by definition, $G_0^{B,R}$ and $G_1^{B,R}$, and the covariance inside the expectation of the second summand has already obtained in (56) and is defined to be $C_{01}^{B,R}$. Using the identities in (S.2) it is straightforward to see that

$$\begin{aligned}E_{\boldsymbol{\mu}}[C_{01}^{B,R}] &= \frac{p}{(n_0+\nu_0)(n_1+\nu_1)}+\frac{(n_0-\nu_0)p}{2n_0^2(n_0+\nu_0)}+\frac{(n_1-\nu_1)p}{2n_1^2(n_1+\nu_1)} \\ &+\frac{\frac{p}{\nu_0}}{n_0+\nu_0}\left(1+\frac{n_0}{n_1+\nu_1}-\frac{\nu_0}{n_0}\right)+\frac{\frac{p}{\nu_1}}{n_1+\nu_1}\left(1+\frac{n_1}{n_0+\nu_0}-\frac{\nu_1}{n_1}\right) \\ &-\frac{2}{(n_0+\nu_0)(n_1+\nu_1)}\left(\nu_0+\nu_1+n_0+n_1\right)\mathbf{m}_0^T\boldsymbol{\Sigma}^{-1}\mathbf{m}_1 \\ &+\frac{\mathbf{m}_0^T\boldsymbol{\Sigma}^{-1}\mathbf{m}_0}{n_0+\nu_0}\left(1+\frac{n_0}{n_1+\nu_1}-\frac{\nu_0}{n_0}+\frac{\nu_0(n_0+n_1+\nu_0)}{n_0(n_1+\nu_1)}\right) \\ &+\frac{\mathbf{m}_1^T\boldsymbol{\Sigma}^{-1}\mathbf{m}_1}{n_1+\nu_1}\left(1+\frac{n_1}{n_0+\nu_0}-\frac{\nu_1}{n_1}+\frac{\nu_1(n_0+n_1+\nu_1)}{n_1(n_0+\nu_0)}\right).\end{aligned} \tag{S.6}$$

On the other hand, from the identities in (S.1),

$$\begin{aligned}\mathrm{Cov}_{\boldsymbol{\mu}}[G_0^{B,R},G_1^{B,R}] &= \frac{-n_0n_1p}{\nu_0\nu_1(n_0+\nu_0)(n_1+\nu_1)}-\frac{(n_0-\nu_0)p}{2\nu_0^2(n_0+\nu_0)} \\ &-\frac{(n_1-\nu_1)p}{2\nu_1^2(n_1+\nu_1)}+\left(\frac{2n_0}{\nu_0(n_0+\nu_0)}+\frac{2n_1}{\nu_1(n_1+\nu_1)}\right)\mathbf{m}_0^T\boldsymbol{\Sigma}^{-1}\mathbf{m}_1 \\ &-\frac{1}{n_0+\nu_0}\left(\frac{n_0}{\nu_0}+\frac{n_0n_1}{\nu_1(n_1+\nu_1)}+\frac{\nu_0n_1}{\nu_1(n_1+\nu_1)}\right)\mathbf{m}_0^T\boldsymbol{\Sigma}^{-1}\mathbf{m}_0 \\ &-\frac{1}{n_1+\nu_1}\left(\frac{n_1}{\nu_1}+\frac{n_0n_1}{\nu_0(n_0+\nu_0)}+\frac{\nu_1n_0}{\nu_0(n_0+\nu_0)}\right)\mathbf{m}_1^T\boldsymbol{\Sigma}^{-1}\mathbf{m}_1.\end{aligned} \tag{S.7}$$

The result follows by using (S.6) and (S.7) in (S.5).

### Section F: Proof of Equation (81)

As in Section D, the law of total covariance yields

$$\begin{aligned} K_0^{BT,R} &= \mathrm{Cov}_{\boldsymbol{\mu},S_n,\mathbf{z},\mathbf{x}}[U_0(\bar{\mathbf{x}}_0,\bar{\mathbf{x}}_1,\mathbf{z}),W(\bar{\mathbf{x}}_0,\bar{\mathbf{x}}_1,\mathbf{x})|\mathbf{z}\in\Psi_0,\mathbf{x}\in\Pi_0] \\ &= \mathrm{Cov}_{\boldsymbol{\mu}}[G_0^{B,R},\delta_{\boldsymbol{\mu}}^2] + E_{\boldsymbol{\mu}}[C_0^{BT,R}], \end{aligned}$$

with $G_0^{B,R}$ and $C_0^{BT,R}$ being defined in in (23) and (60), respectively. From identities in (S.1), we get

$$\mathrm{Cov}_{\boldsymbol{\mu}}[G_0^{B,R},\delta_{\boldsymbol{\mu}}^2] = \left(\frac{1}{\nu_1} + \frac{n_0}{\nu_0(n_0+\nu_0)}\right)\Delta_{\mathbf{m}}^2 + \frac{(n_0-\nu_0)p}{2\nu_0^2(n_0+\nu_0)} + \frac{n_0 p}{\nu_0\nu_1(n_0+\nu_0)} + \frac{p}{2\nu_1^2}.$$

$E_{\boldsymbol{\mu}}[C_0^{BT,R}]$ is obtained using (S.2) and the result follows.

### Section G: Proof of Equation (83)

As in Section E, the law of total covariance yields

$$\begin{aligned} K_{01}^{BT,R} &= \mathrm{Cov}_{\boldsymbol{\mu},S_n,\mathbf{z},\mathbf{x}}[U_0(\bar{\mathbf{x}}_0,\bar{\mathbf{x}}_1,\mathbf{z}),-W(\bar{\mathbf{x}}_0,\bar{\mathbf{x}}_1,\mathbf{x})|\mathbf{z}\in\Psi_0,\mathbf{x}\in\Pi_1] \\ &= -\mathrm{Cov}_{\boldsymbol{\mu}}[G_0^{B,R},-\delta_{\boldsymbol{\mu}}^2] + E_{\boldsymbol{\mu}}[C_{01}^{BT,R}], \end{aligned}$$

where $C_{01}^{BT,R}$ is presented in (64). $\mathrm{Cov}_{\boldsymbol{\mu}}[G_0^{B,R},\delta_{\boldsymbol{\mu}}^2]$ has been obtained in Section F, $E_{\boldsymbol{\mu}}[C_{01}^{BT,R}]$ follows from the identities in (S.2), and by some algebraic manipulations yield the result.

## 2. Supplementary Figures, Tables, and Experiments

### Figures

Here, we consider the accuracy of finite-sample approximations obtained directly from theorems rather than considering Raudys-type of finite-sample approximations. In Figure S1 we consider the approximations directly suggested by the theorems. The RMS is not included because the corresponding approximation coming directly from theorems for the unconditional case is identically 0. Figure S1 compares the first moments obtained from Theorems 1 and 2, equations (17) and (30), to Monte Carlo estimation of the first moment of $\hat{\varepsilon}^B$. It presents $E_{S_n}[\hat{\varepsilon}^B|\boldsymbol{\mu}]$ and $E_{\boldsymbol{\mu},S_n}[\hat{\varepsilon}^B]$ computed by Monte Carlo estimation and the analytical expressions. The label "asym BE Uncond" identifies the curve of $E_{\boldsymbol{\mu},S_n}[\hat{\varepsilon}^B]$, the unconditional expected estimated error, which according to the basic theorey is equal to $E_{\boldsymbol{\mu},S_n}[\varepsilon]$. The labels "asym BE Cond" and "asym TE Cond" show the curves of $E_{S_n}[\hat{\varepsilon}^B|\boldsymbol{\mu}]$, the conditional expected estimated error, and $E_{S_n}[\varepsilon|\boldsymbol{\mu}]$, the conditional expected true error, respectively, both obtained using the analytic approximations obtained from asymptotic results. The plots show substantial agreement with the Monte Carlo approximation.

Figure S2-S3 compare finite-sample approximations obtained from Theorems 3-6, equations (39), (42), (45), (71), and (72) to Monte Carlo estimation of the conditional and unconditional second/mixed moments. The labels are interpreted similarly to those in S1, but for the second/mixed moments instead. The figures show that the finite-sample approximations for the conditional and unconditional second/mixed moments are quite accurate (close to the MC value). The asymptotic approximations of $E_{\boldsymbol{\mu},S_n}[\hat{\varepsilon}^B\varepsilon]$ and $E_{\boldsymbol{\mu},S_n}[\varepsilon^2]$ are not plotted because these approximations are equivalent to that of $E_{\boldsymbol{\mu},S_n}[(\hat{\varepsilon}^B)^2]$. However, the figures shows that the MC estimations of $E_{\boldsymbol{\mu},S_n}[\hat{\varepsilon}^B\varepsilon]$, $E_{\boldsymbol{\mu},S_n}[\varepsilon^2]$, and $E_{\boldsymbol{\mu},S_n}[(\hat{\varepsilon}^B)^2]$ are extremely close.

The plots in Figure S3 show that the finite-sample approximations obtained directly from Theorems 1-6 are very accurate for the conditional case, $\mathrm{RMS}_{S_n}[\hat{\varepsilon}^B|\boldsymbol{\mu}]$, but the unconditional case is a problem for the analytical approximations, because here, according to (72), we have unconditional variance of true error and Bayesian estimator, unconditional deviation variance, and unconditional RMS, all asymptotically identical to 0 and we need to use the Raudys-type of finite sample approximations (see Figure 1).

Table 1: Minimum sample size, $n$, ($n_0 = n_1 = \frac{n}{2}$) to satisfy $\kappa_{\hat{\varepsilon}}(n, p, \beta) < \tau$ (conditional case).

| $\tau$ | p = 2 | p = 4 | p = 8 | p = 16 | p = 32 | p = 64 | p = 128 |
|---|---|---|---|---|---|---|---|
| $\beta = 0.5$ | | | | | | | |
| 0.1 | 26 | 40 | 68 | 124 | 234 | 456 | 898 |
| 0.09 | 32 | 50 | 84 | 152 | 290 | 564 | 1114 |
| 0.08 | 42 | 64 | 108 | 194 | 370 | 718 | 1416 |
| 0.07 | 56 | 84 | 142 | 256 | 484 | 940 | 1856 |
| 0.06 | 76 | 116 | 194 | 350 | 662 | 1284 | 2532 |
| 0.05 | 112 | 168 | 280 | 504 | 954 | 1854 | 3654 |
| $\beta = 1$ | | | | | | | |
| 0.1 | 14 | 22 | 38 | 70 | 132 | 256 | 506 |
| 0.09 | 18 | 28 | 48 | 86 | 164 | 318 | 626 |
| 0.08 | 24 | 36 | 60 | 110 | 208 | 404 | 796 |
| 0.07 | 32 | 48 | 80 | 144 | 272 | 530 | 1044 |
| 0.06 | 44 | 64 | 108 | 196 | 372 | 722 | 1424 |
| 0.05 | 62 | 94 | 158 | 284 | 538 | 1044 | 2056 |
| $\beta = 2$ | | | | | | | |
| 0.1 | 6 | 10 | 16 | 30 | 58 | 114 | 224 |
| 0.09 | 8 | 12 | 22 | 38 | 72 | 142 | 278 |
| 0.08 | 10 | 16 | 26 | 48 | 92 | 180 | 354 |
| 0.07 | 14 | 22 | 36 | 64 | 122 | 236 | 464 |
| 0.06 | 20 | 28 | 48 | 88 | 166 | 322 | 634 |
| 0.05 | 28 | 42 | 70 | 126 | 238 | 464 | 914 |

## Tables

Table 1 shows the minimum number of sample points needed to guarantee having a predetermined conditional RMS for the whole range of $\delta^2_{\boldsymbol{\mu}}$.

Table 2 shows the minimum sample size that guarantees having a predetermined unconditional RMS for the whole range of $\Delta^2_{\mathbf{m}}$.

Table 2: Minimum sample size, $n$, ($n_0 = n_1 = \frac{n}{2}$) to satisfy $\kappa_{\hat{\varepsilon}}(n, p, \beta) < \tau$ (unconditional case).

| $\tau$ | p = 2 | p = 4 | p = 8 | p = 16 | p = 32 | p = 64 | p = 128 |
|---|---|---|---|---|---|---|---|
| $\beta = 0.5$ | | | | | | | |
| 0.025 | 88 | 86 | 80 | 68 | 2 | 2 | 2 |
| 0.02 | 142 | 138 | 134 | 122 | 94 | 2 | 2 |
| 0.015 | 256 | 254 | 248 | 236 | 212 | 148 | 2 |
| 0.01 | 584 | 582 | 576 | 564 | 542 | 494 | 374 |
| 0.005 | 2370 | 2358 | 2348 | 2336 | 2312 | 2268 | 2178 |
| $\beta = 1$ | | | | | | | |
| 0.025 | 108 | 108 | 106 | 102 | 92 | 72 | 2 |
| 0.02 | 172 | 170 | 168 | 164 | 156 | 138 | 78 |
| 0.015 | 308 | 306 | 304 | 300 | 292 | 274 | 236 |
| 0.01 | 694 | 694 | 690 | 686 | 678 | 662 | 628 |
| 0.005 | 2790 | 2786 | 2782 | 2776 | 2768 | 2752 | 2720 |
| $\beta = 2$ | | | | | | | |
| 0.025 | 82 | 82 | 80 | 80 | 76 | 70 | 56 |
| 0.02 | 128 | 128 | 126 | 126 | 122 | 118 | 104 |
| 0.015 | 228 | 228 | 228 | 226 | 224 | 218 | 206 |
| 0.01 | 514 | 514 | 514 | 512 | 510 | 504 | 494 |
| 0.005 | 2064 | 2062 | 2062 | 2060 | 2058 | 2052 | 2042 |

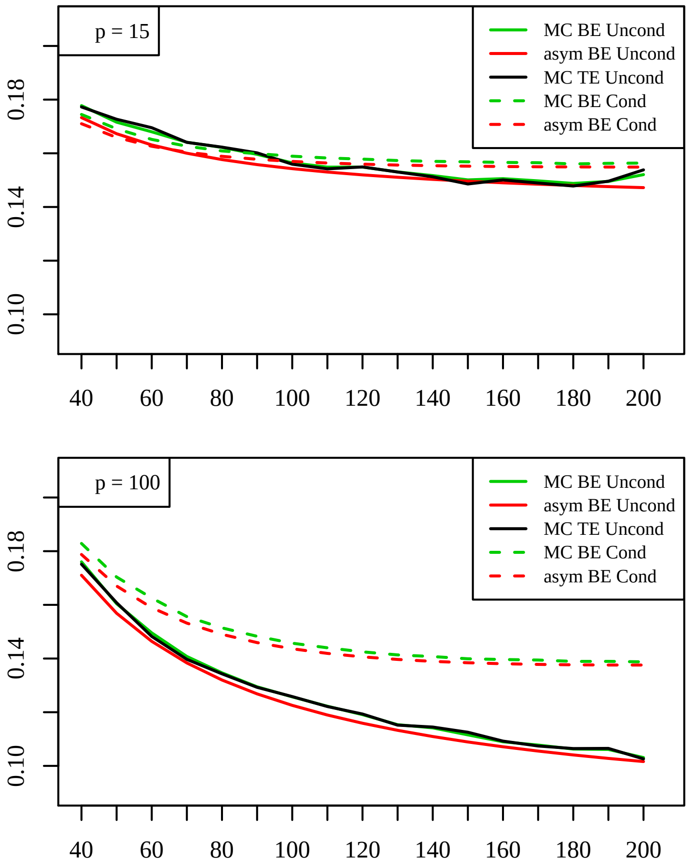


Figure S1: Comparison of expectation of $\hat{\varepsilon}^B$ using asymptotically exact finite setting approximations, with Monte Carlo estimates as a function of sample size for dimensions p = 15 and 100, for $\nu_0 = \nu_1 = 50$, $\mathbf{m}_i = \boldsymbol{\mu}_i + 0.01\boldsymbol{\mu}_i$ with $\boldsymbol{\mu}_0 = -\boldsymbol{\mu}_1$ (Bayes error 0.1586). The case of asymptotic unconditional expectation of $\varepsilon$ is not plotted because $\lim_{\text{b.k.a.c.}} \text{Bias}_{U,n}[\hat{\varepsilon}^B] = 0$.

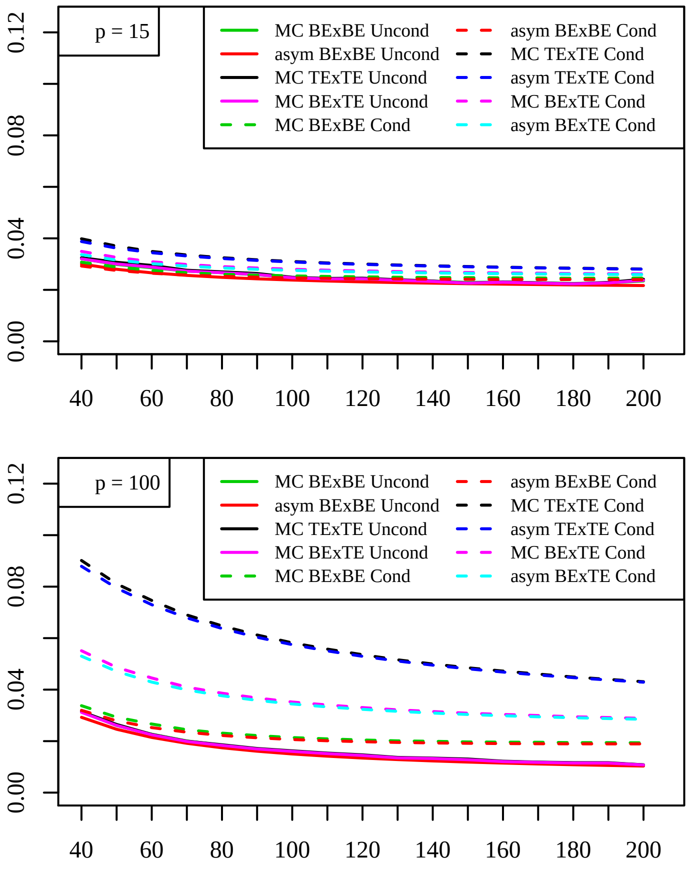


Figure S2: Comparison of conditional and unconditional second and mixed moments using asymptotically exact finite setting approximations with Monte Carlo estimates as a function of sample size for dimensions p = 15 and 100, for $\nu_0 = \nu_1 = 50$, $\mathbf{m}_i = \boldsymbol{\mu}_i + 0.01\boldsymbol{\mu}_i$ with $\boldsymbol{\mu}_0 = -\boldsymbol{\mu}_1$ (Bayes error 0.1586). The case of asymptotic approximations of $E_{\boldsymbol{\mu},S_n}[\hat{\varepsilon}^B\varepsilon]$ and $E_{\boldsymbol{\mu},S_n}[\varepsilon^2]$ are not plotted as their analytical approximations are equivalent to that of $E_{\boldsymbol{\mu},S_n}[(\hat{\varepsilon}^B)^2]$ (see (71)).

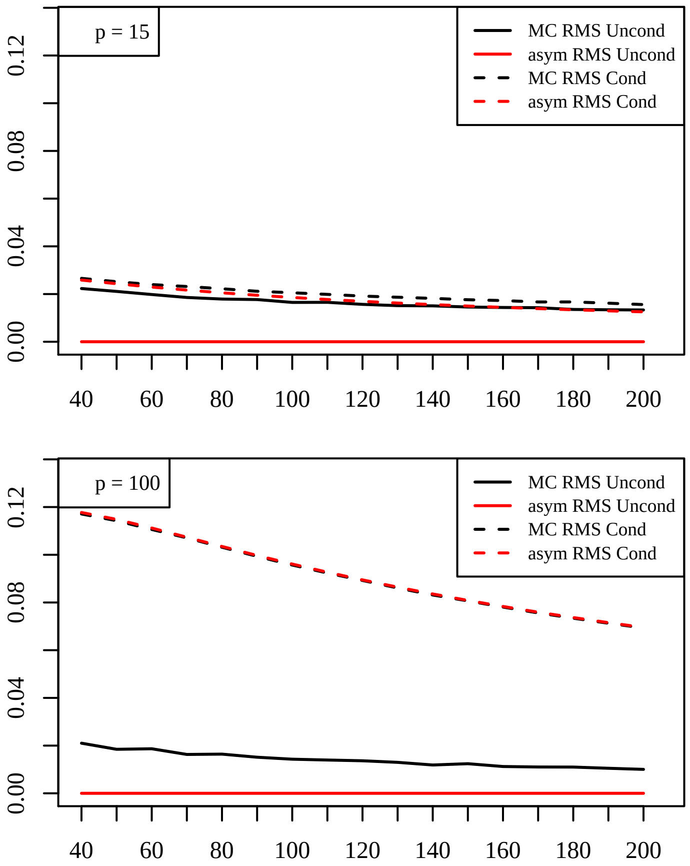


Figure S3: Comparison of conditional RMS, i.e. $\mathrm{RMS}_{S_n}[\hat{\varepsilon}^B|\boldsymbol{\mu}]$ and, unconditional RMS, i.e. $\mathrm{RMS}_{\boldsymbol{\mu},S_n}[\hat{\varepsilon}^B]$, using asymptotically exact finite setting approximations, with Monte Carlo estimates as a function of sample size for dimensions p = 15 and 100, for $\nu_0 = \nu_1 = 50$, $\mathbf{m}_i = \boldsymbol{\mu}_i + 0.01\boldsymbol{\mu}_i$ with $\boldsymbol{\mu}_0 = -\boldsymbol{\mu}_1$ (Bayes error 0.1586).

## Experiments

To examine the accuracy of the required sample size that satisfies $\kappa_{\hat{\varepsilon}}(n, p, \beta) < \tau$ for both conditional and unconditional settings, we performed the following set of experiments.

We used Table 1 to determine the minimum number of sample points needed to achieve $\tau = 0.1, 0.07, 0.05$ for conditional RMS, and $\tau = 0.025, 0.015, 0.005$ for the unconditional RMS for $p = 8, 32$, and $\beta = 1$. We used Monte-Carlo simulations according to protocol presented in Section 6, and plotted the curves of RMS versus the class distances. Class distance is determined by $\delta^2_{\boldsymbol{\mu}}$ for conditional case, and with $\Delta^2_{\mathbf{m}}$ for unconditional case. For the conditional case and for equal mixing probability of classes, $\delta^2_{\boldsymbol{\mu}}$ determines the Bayes error according to $\epsilon_{Bayes} = \Phi(-\frac{\delta_{\mu}}{2})$. Figure S4 shows the result of this analysis. Clearly, the RMS curves in both conditional and unconditional cases are below the RMS thresholds for the whole range of class distance. These results show that the minimum required sample points tabulated in Table 1 can accurately determine the number of sample points needed to assure having a predetermined maximum tolerable level of RMS regardless of the class distance.

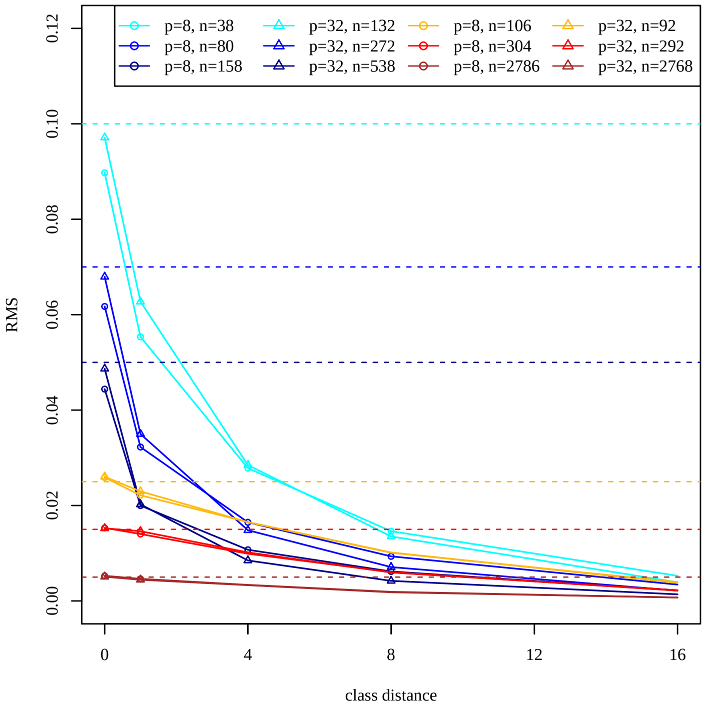


Figure S4: Conditional (unconditional) RMS as a function of class distance, i.e. $\delta^2_{\boldsymbol{\mu}}$ ($\Delta^2_{\mathbf{m}}$). The dashed lines identify the required threshold for RMS, i.e. $\tau$. The three dashed lines on the top identify the limits for conditional RMS, $\tau = 0.1, 0.07, 0.05$, respectively. As expected, the curves of conditional RMS versus $\delta^2_{\boldsymbol{\mu}}$ identified by $p = 8, n = 38$ and $p = 32, n = 132$; $p = 8, n = 80$ and $p = 32, n = 272$; and $p = 8, n = 158$ and $p = 32, n = 538$ are below $\tau = 0.1$, $\tau = 0.07$, and $\tau = 0.05$, respectively. The three dashed lines at the bottom identify the limits for unconditional RMS, $\tau = 0.025, 0.015, 0.005$, respectively. As expected, the curves of unconditional RMS versus $\Delta^2_{\mathbf{m}}$ identified by $p = 8, n = 106$ and $p = 32, n = 92$; $p = 8, n = 304$ and $p = 32, n = 292$; and $p = 8, n = 2786$ and $p = 32, n = 2768$ are below $\tau = 0.025$, $\tau = 0.015$, and $\tau = 0.005$, respectively.

## References

[1] R. Kan, "From moments of sum to moments of product," *J. Multivariate Anal.*, vol. 99, pp. 542 – 554, 2008.
